# Supplementary material for: Efficient Recovery Learning using Model Predictive Meta-Reasoning
Source: arXiv:2209.13605 source file (2023-03-09)
Supplement: Supplementary file 1 [file 8_appendix.tex]

\begin{appendices}
\normalsize
\section{Approach}
\subsection{Precondition Chaining}
\begin{algorithm}
\centering
    \begin{algorithmic}[1]
        \Procedure{PreconditionChaining}{$\{\pi^0_1, \cdots,\pi^0_k\}$}
        % Estimate positive distribution
        \State{Execute skill chain and collect N successful trajectories of size $k+1$}
        \State{$\mathcal{D}^+_{1:k} \leftarrow$ Learn positive distribution of the start of every skill}
        \State{goal $\leftarrow f_{goal}$} \Comment{Overall task goal}
        \For{$i \in \{k, k-1,\cdots,1\}$} \Comment{backwards from goal}
            \State{$X \leftarrow \phi, Y \leftarrow \phi$}
            \For{$1\leq j \leq M$}
                \State{Sample $\tau$ from $\mathcal{D}^+_i$}
                \State{Set state to $\tau$ and execute $\pi_i^0$}
                \State{y $\leftarrow 1$ if goal is satisfied, 0 otherwise}
                \State{$X = X \cup \tau$, $Y = Y \cup y$}
                %\If{\textsc{success}}
                %\EndIf
            \EndFor
            \State{$\rho_i \leftarrow$ Train classifier using $(X, y)$}
            \State{goal $\leftarrow \rho_i$}
        \EndFor
            \Return{$\{\rho_1,\cdots,\rho_k\}$}
        \EndProcedure
    \end{algorithmic}
    \caption{Learning the preconditions of nominal skills via precondition chaining.}
    \label{alg:precond_chaining}
\end{algorithm}

\begin{figure*}[th]
    \centering
    \includegraphics[width=0.8\textwidth]{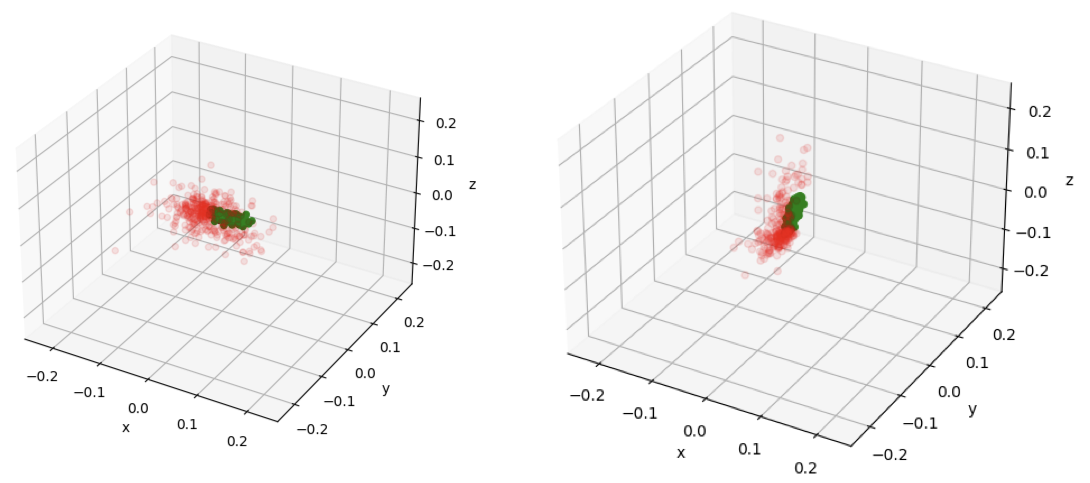}
    \caption{We show the data used to train preconditions.
    Note that we only plot the end-effector position with respect to the handle.
    Positive samples are shown in green, while negative samples are shown in red.
    \emph{(left)} Precondition for \textsc{RotateHandle} skill.
    The positive samples are distributed horizontally along the handle.
    \emph{(right} Precondition for the \textsc{PullHandle} skill.
    The positive samples are distributed along the handle which is vertical.
    }
    \label{fig:preconds}
\end{figure*}

% \subsection{Markov Decision Process}

\section{Experiments}
\subsection{Evaluation in Simulation}
We modified the door and handle properties to match the real handle that we use.
In particular, we make the handle smaller, lower friction values and increase the spring constants of the door and handle joints.
These changes make the task harder than the robosuite version but better match our real handle.
\begin{figure}[t]
\centering
\includegraphics[width=1\columnwidth]{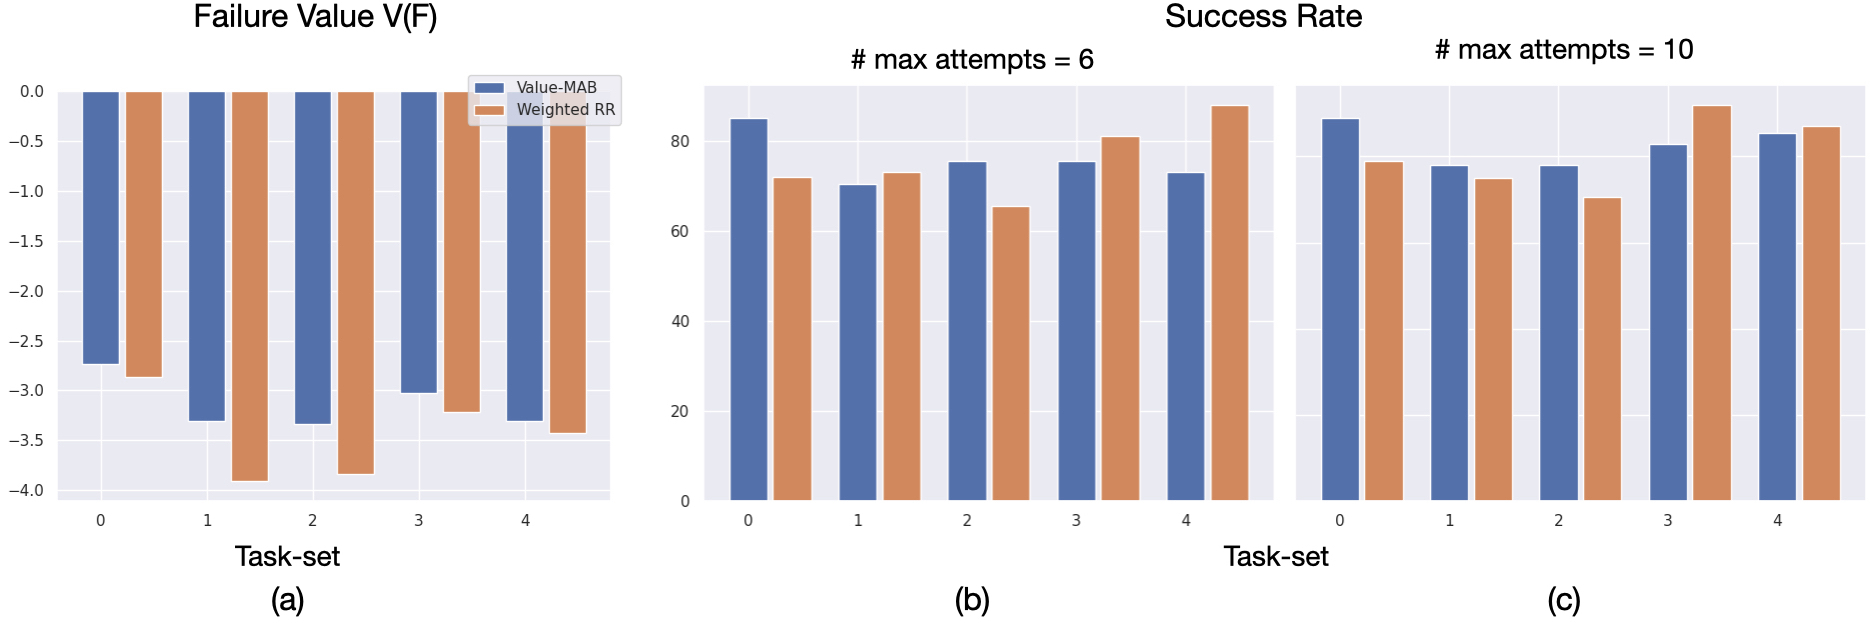}\vspace{-5mm}
\label{fig:results}
\caption{Comparison between Value-MAB and Weighted RR on 5 task-sets:
\emph{(a)} \emph{Failure Value:}
Value-MAB consistently achieves higher $V(F)$ as it directly optimizes it during allocation.
Next, we evaluate the success rate of nominal and recovery skills in simulation by executing them with a state estimator.
\emph{(b)} Each evaluation is limited to 6 skill executions.
There is no significant difference in success rate.
\emph{(c)} Each attempt is limited to 10 skill executions.
Value-MAB performs better than weighted RR on average.
% \vspace{-5mm}
}
\end{figure}

% \subsection{Ablation}

% \subsection{Evaluation on a Real Robot}
\begin{figure}[t]
    \centering
    \includegraphics[width=1.0\textwidth]{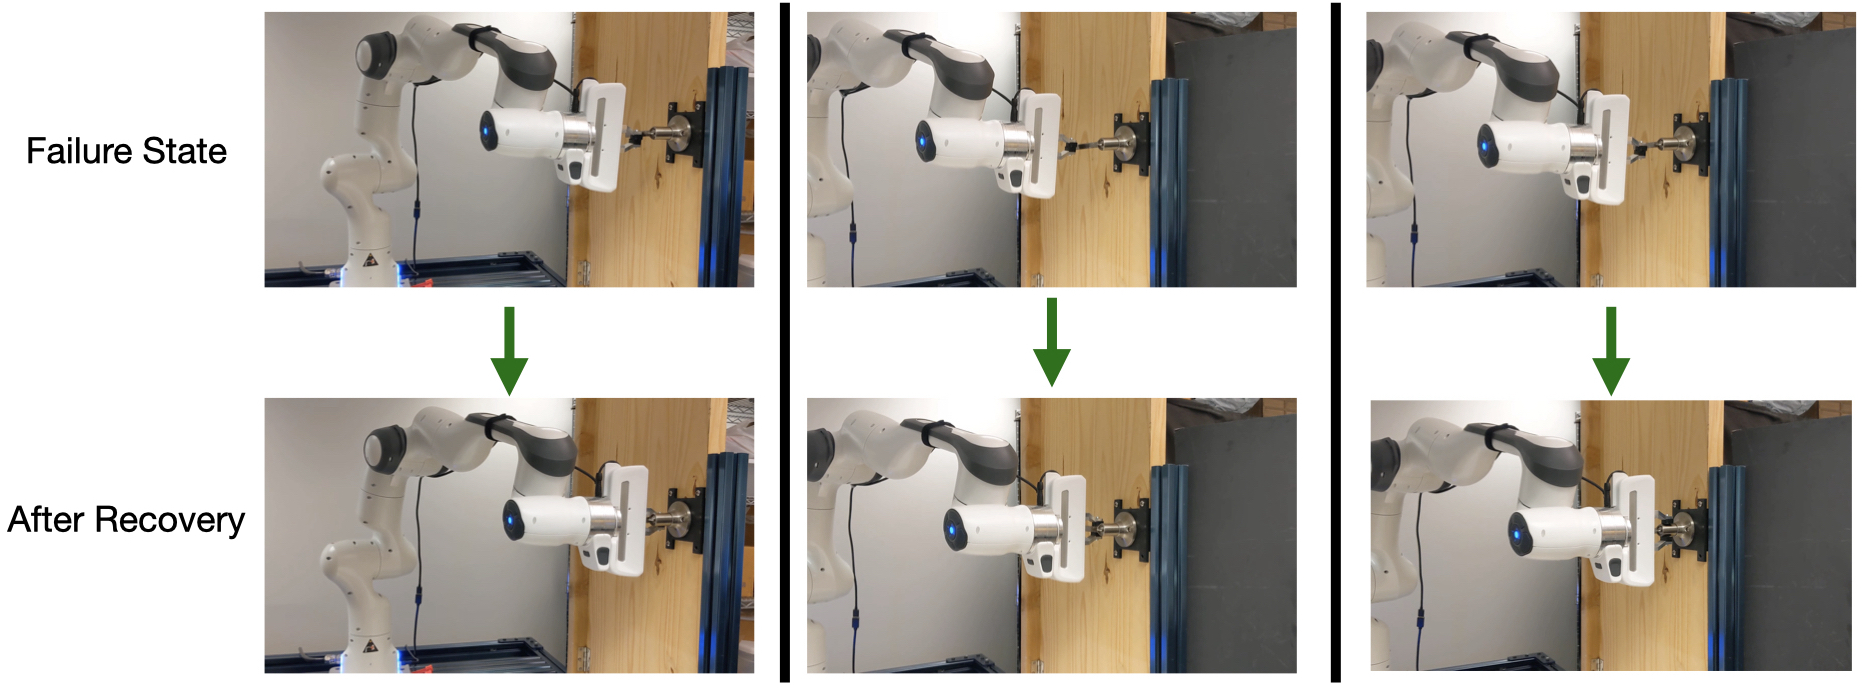}
    \caption{We show three failures encountered in our experiments.
    \emph{(top)} Robot ends up in failure states due to incorrect handle position.
    \emph{(bottom)} The robot re-grasps the handle to recover from the failure.
}
    \label{fig:failure_vs_recovery}
\end{figure}

% \subsection{Common Failure Modes}
% \textcolor{red}{TODO: Explain where and why failure recovery fails.}
% 
% - better sensing is needed to track the pose of the handle once it is occluded.

\section{Implementation Details}
\subsection{Preconditions}
Each precondition is  a generative classifier with the positive distribution learnt using a Gaussian distribution and the negative distribution learnt using a Gaussian Mixture Model with 4 components.
To learn a tight decision boundary, we
\begin{enumerate}
    \item First learn an initial positive distribution for each precondition by executing nominal skills from the start state.
    \item During precondition chaining, we sample additional states in the neighbourhood of each positive distribution by scaling its covariance matrix and sampling from it.
    \item We sample random world states and treat them as negative data-points for all preconditions.
\end{enumerate}

\subsection{Relative Entropy Policy Search (REPS)}
We use REPS~\cite{peters2010relative} as our oracle  to generate trajectories which are used to learn recovery skills.
REPS is a policy search algorithm for control problems that seeks to improve the policy based on past trials.
The key feature is that instead of using a fixed step size in policy update, REPS constrains the loss of information (relative entropy) due to policy update.
In our experiment, we use a relative entropy bound of 0.5.
We perform a total of 10 policy updates for every oracle call, where, each policy update is based on 40 experiences collected with the current policy.

% \subsection{Multi}

% \subsection{Nominal Skills}
% Each nominal skill is a hand-designed
% \subsection{Environment}
% \textbf{State Space}
% \begin{itemize}
%     \item Handle pose: position (3) + angle (1) = 4 dims
%     \item Door angle: 1 dims
%     \item Robot joints: 7 dims
%     \item 
% \end{itemize}

% \subsection{Context Space}
% \begin{itemize}
%     \item  Handle dimensions: 3
%     \item Handle mass: 1
%     \item Handle friction: 1
%     \item Door mass: 1
% \end{itemize}

% \subsection{Nominal Skills}
% We provide a detailed description of our nominal skills:

% \begin{enumerate}
%     \item \textbf{\textsc{GoToHandle}}
%     \item \textbf{\textsc{GraspHandle}}
%     \item \textbf{\textsc{RotateHandle}}
%     \item \textbf{\textsc{PullHandle}}
% \end{enumerate}

\end{appendices}
